# Supplementary material for: Differential branching fraction and angular moments analysis of the decay $B^0 \to K^+ \pi^- \mu^+ \mu^-$ in the $K^*_{0,2}(1430)^0$ region
Source: arXiv:1609.04736 source file (2016-12-22)
Supplement: Supplementary file 1 [file supplementary-app.tex]

\clearpage
\setcounter{secnumdepth}{0}
\section{Supplementary material for LHCb-PAPER-2016-025}
\label{sec:Supplementary-App}

% This appendix contains supplementary material that will be posted
% on the public cds record but will not appear in the paper.

\subsection{Normalised moments and covariance matrix}

The normalised moments, $\overline{\Gamma}_{i}$, and corresponding covariance matrix, $\overline{C}_{ij}$, are included in a supplementary file \texttt{LHCb-PAPER-2016-025-supplementary.txt}. The covariance matrix contains contributions from both the statistical and systematic uncertainties. As the statistical errors are dominant, the systematic uncertainties are treated as uncorrelated.

\clearpage
